# Supplementary material for: MELINDA: A Multimodal Dataset for Biomedical Experiment Method Classification
Source: arXiv:2012.09216 source file (2020-12-16)
Supplement: Supplementary file 1 [file appendix_data_top_k_words.tex]

\begin{figure}[ht!]
\centering
    \includegraphics[width=\columnwidth]{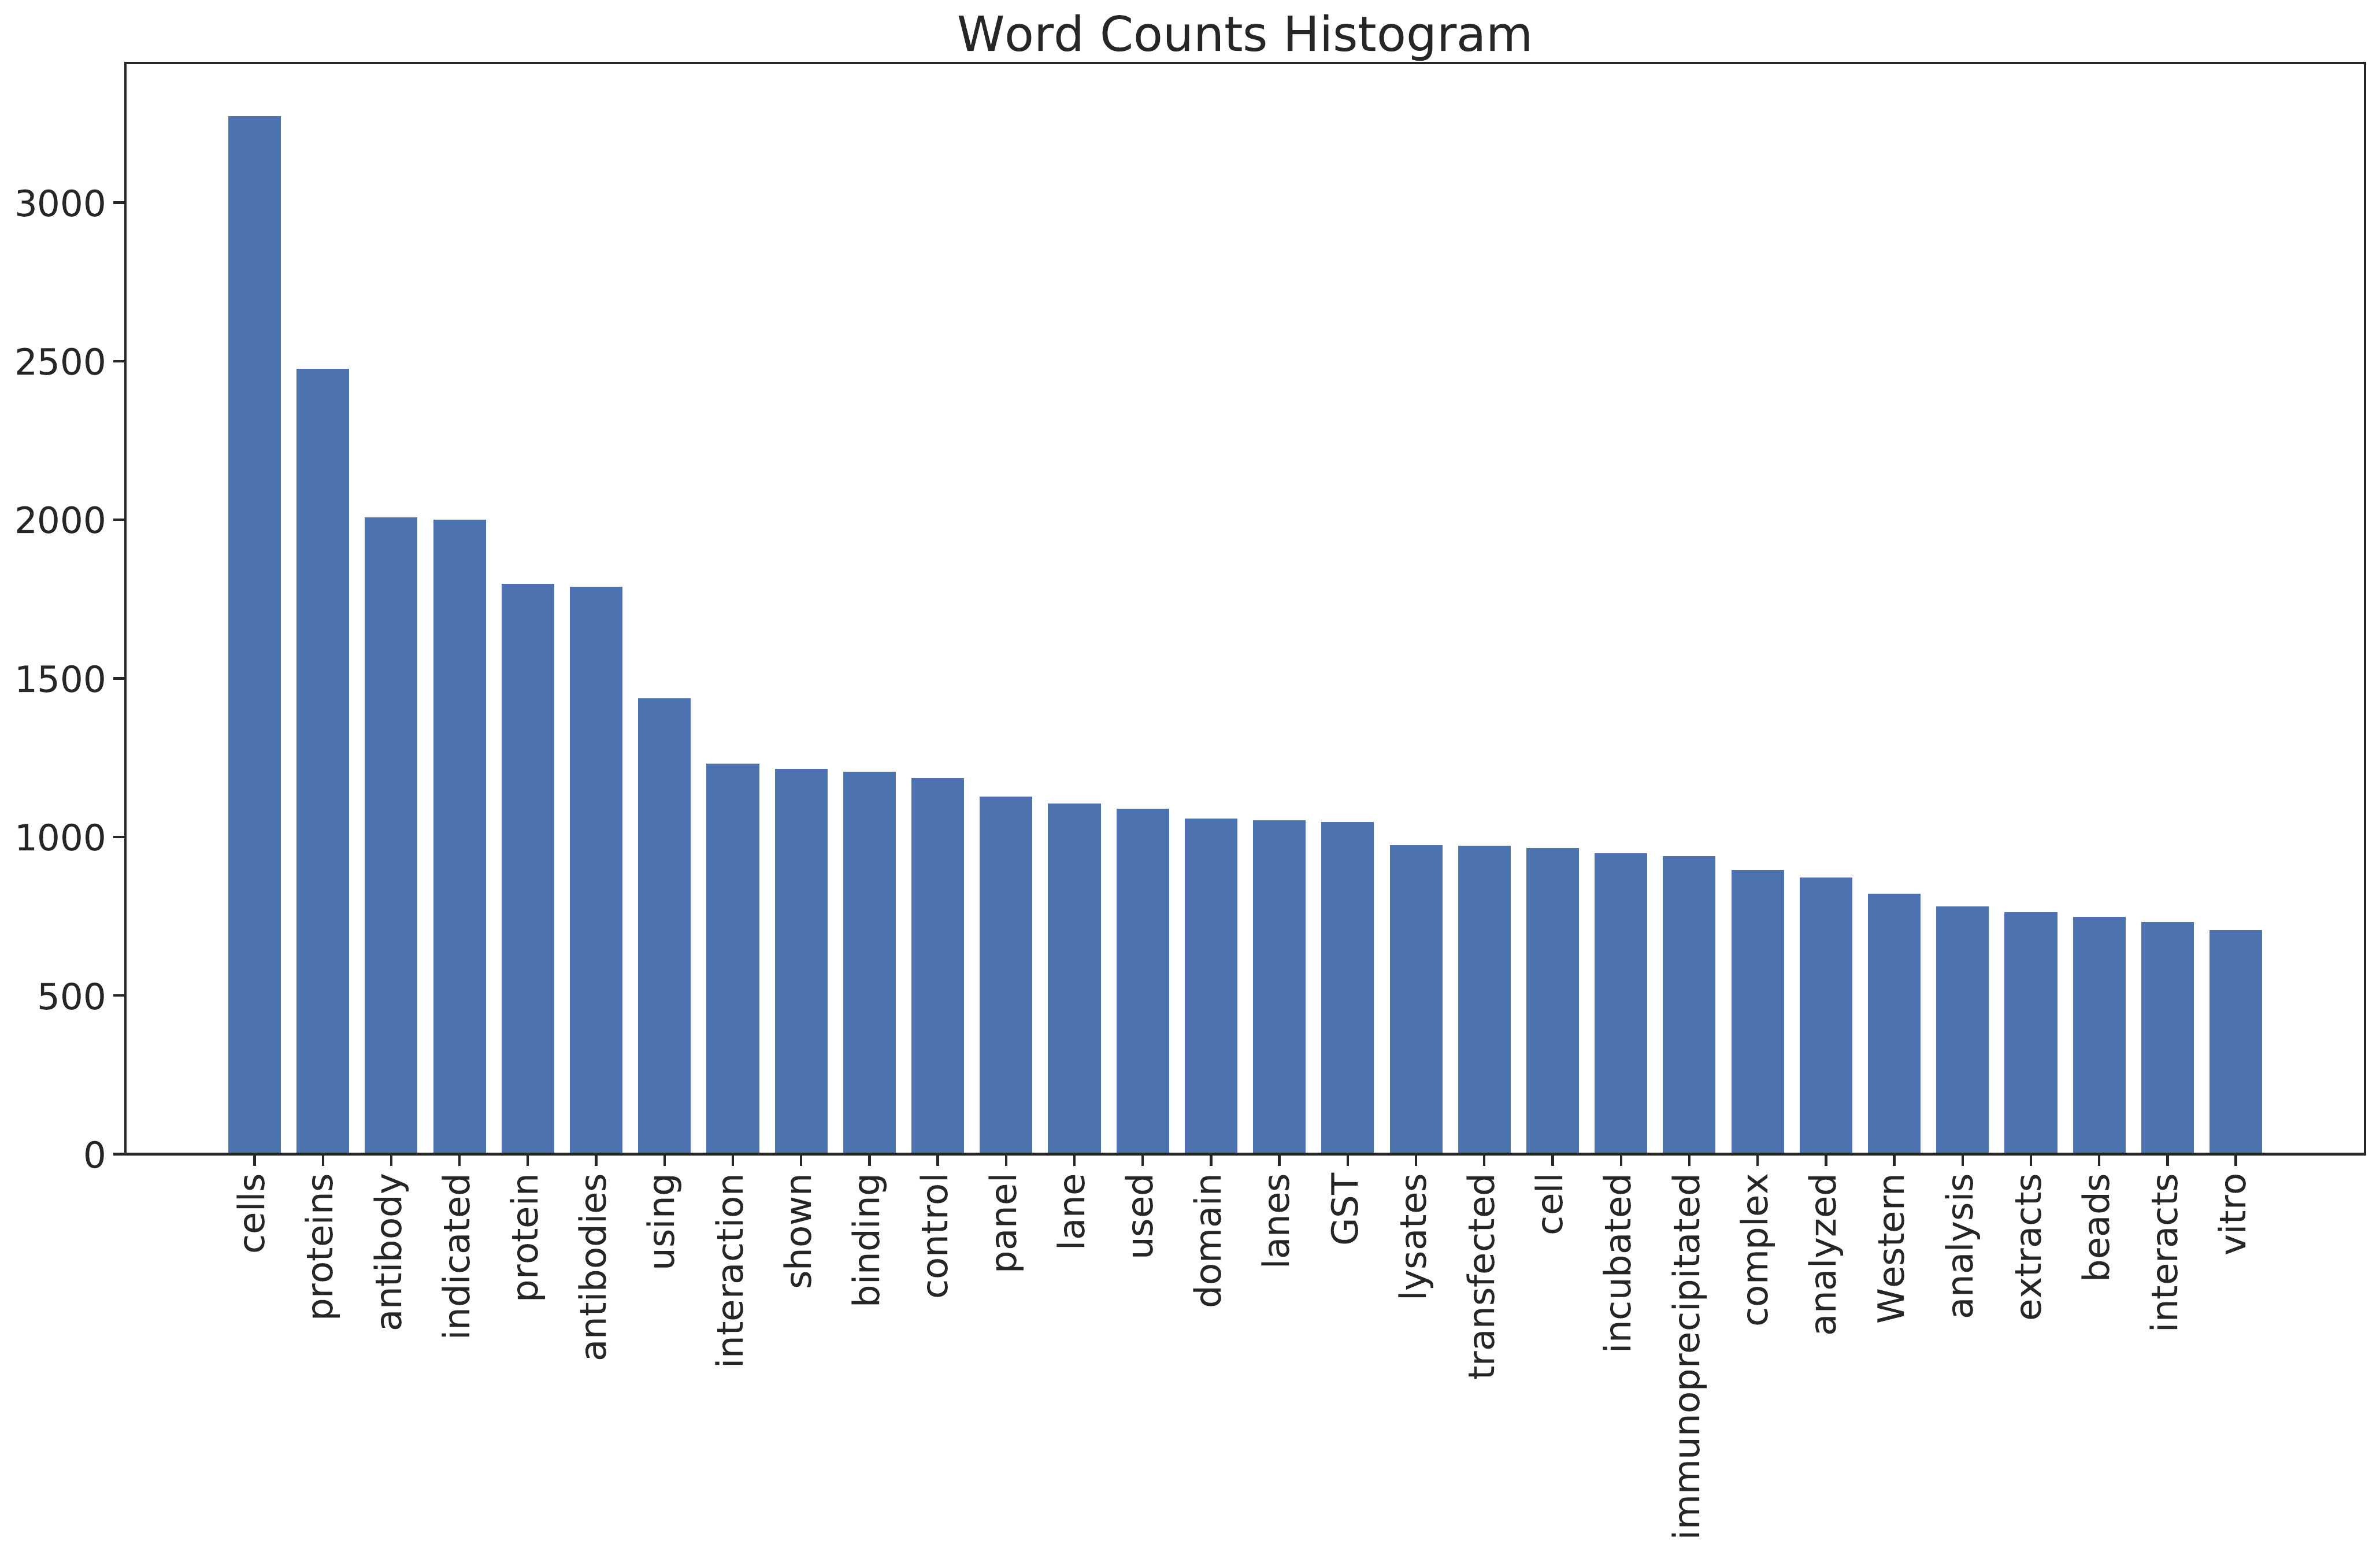}
    \caption{
        Top-30 frequent words (\telin{to be fine-tuned}): captions go here.
    }
    \label{fig:appendix_data_topk1}
\end{figure}

\begin{figure}[ht!]
\centering
    \includegraphics[width=\columnwidth]{figs/imgs/total_word_counts_hist.pdf}
    \caption{
        Top-30 frequent words (\telin{to be fine-tuned}): captions go here.
    }
    \label{fig:appendix_data_topk2}
\end{figure}
