# Supplementary material for: MELINDA: A Multimodal Dataset for Biomedical Experiment Method Classification
Source: arXiv:2012.09216 source file (2020-12-16)
Supplement: Supplementary file 3 [file obj_detected.tex]

\begin{figure}[ht!]
\centering
    \includegraphics[width=0.6\columnwidth]{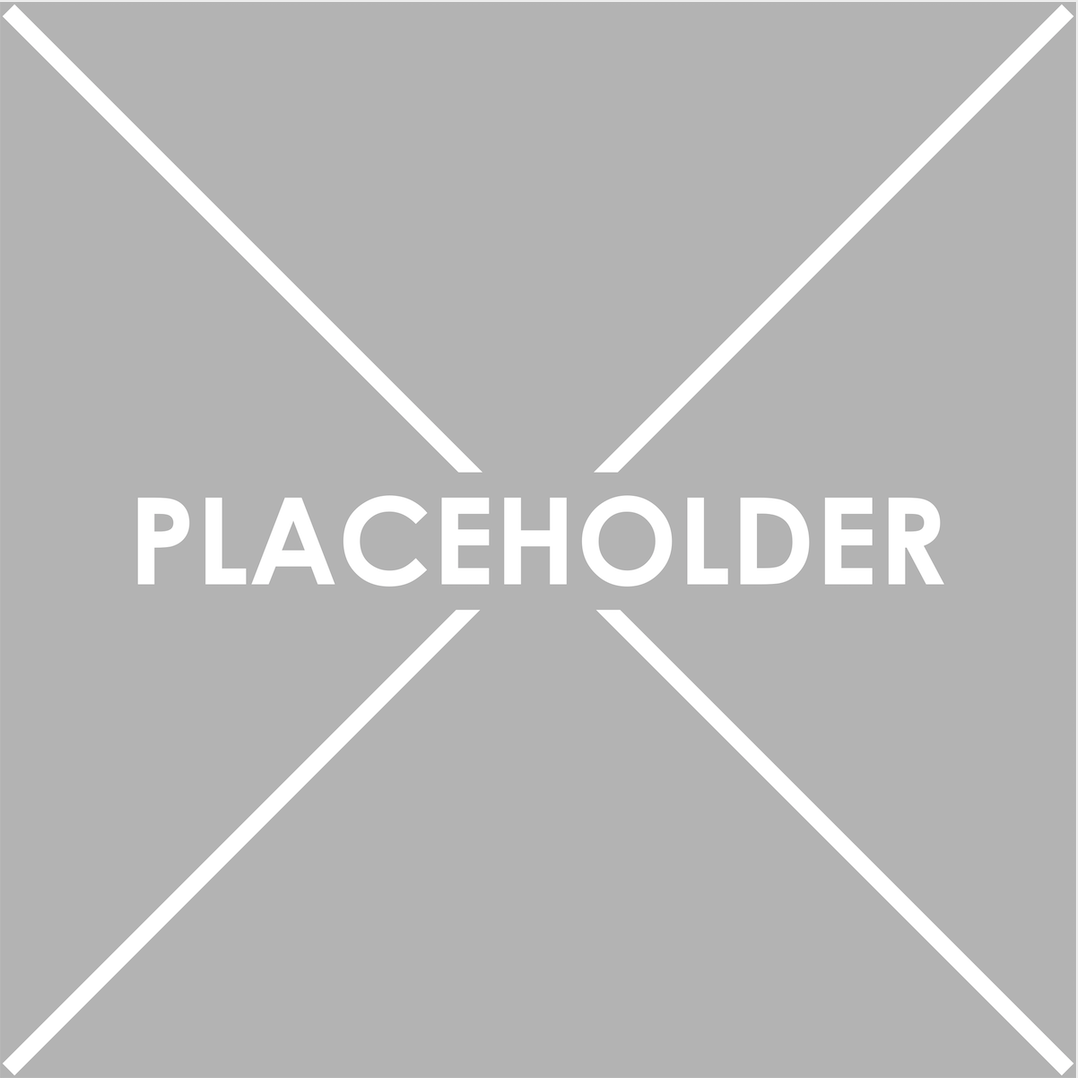}
    \caption{
        \textbf{Detected objects in images of \dataset:} we show some examples of the detected and proposed ROIs from off-the-shelf state-of-the-art object detection modules (\ie detectron2 from FAIR), on the images in~\dataset. One can notice that \telinred{finish}
    }
    \label{fig:appendix_obj_detect}
\end{figure}
